# Supplementary material for: Rethinking Generative Reconstruction Attacks against Graph Neural Network Models
Source: arXiv:2606.29748 source file (2026-06-29)
Supplement: Supplementary file 1 [file appendix.tex]

\section{Appendix}
\label{sec:app}

This is the supplementary document containing the additional results and details of our XXX, as well as cluster details and additional preliminaries.
